# Supplementary material for: DialogStudio: Towards Richest and Most Diverse Unified Dataset Collection for Conversational AI
Source: arXiv:2307.10172 source file (2024-02-05)
Supplement: Supplementary file 1 [file appendix_tod.tex]

\section{Processing for TOD Datasets} \label{sec:appendix_tod}
\subsection{ABCD}
\subsection{AirDialogue}
\subsection{BiTOD}
\subsection{CaSiNo}
\subsection{CraiglistBargains}
\subsection{DSTC2}
\subsection{FRAMES}
\subsection{Key-Value Retrieval Environment for Task-oriented Dialogue (KVRET)}
For each dialogue in the dataset, we extract the domain, and initialize a new dialogue dictionary with some metadata. We then iterate over each turn in the dialogue. If the turn is from the "driver" (user), we create a new turn dictionary and add the user's utterance and other annotations. If the turn is from the "assistant", we add the system's response and other annotations. We also construct the DST and DST ACC (accumulated DST) fields, which hold the current state of the dialogue regarding slots and values. If the turn includes certain slot types ("poi" or "event"), we add the slot value to the result list.

% Dialogue and Turn Formatting: The original dialogues and turns are represented in a new, potentially more convenient format. For each dialogue, a new ID is created, and it also includes some original information like scenario UUID. Each turn in the dialogue is given a new format with fields like USR-UTT, SYS-UTT, DIAL-HIST, DST, DST-ACC, and others.

% Dialogue History: For each turn, the code constructs a DIAL-HIST field, which is a string representation of all previous utterances in the dialogue up to that point.

% Slot-Value Formatting: The original slot-value annotations are converted into a string format in the DST field, and the accumulated slot-value pairs up to each turn are stored in the DST-ACC field.

% External Knowledge Representation: The code also constructs representations of the external knowledge associated with each dialogue. For the task-oriented dialogue (TOD) task, it selects the relevant items from the original KB items and stores them in the EK-ORI field. For the dialogue state tracking (DST) task, it includes the possible slot values from the schema in the EK-ORI field. It then turns these dictionaries into string representations in the EK, EK-DST, and EK-INTENT fields.

% Prompt Generation: The code adds a PROMPT field to each dialogue, which is a generated prompt for that dialogue based on its domain.

\subsection{MetaLWOZ}
\subsection{MSDC}
\subsection{MuDoCo}
\subsection{MulDoGo}
\subsection{MultiWOZ}
\subsection{SalesBot}
\subsection{Schema-Guided Dialogue (SGD)}
% Introduction to the dataset
The SGD dataset consists of over 20,000 dialogues spanning 26 services across 16 domains. These domains range from restaurants and hotels to weather and music. Each dialogue in the dataset contains annotations for user and system utterances, dialogue states, and dialogue acts.

Each turn in this dataset is well annotated with dialog states, for both slots from the current turn and accumulated slots so far. Therefore, we extract the current turn slot from $turn[``frames"][``slots"]$ and accumulated slots from $turn[``frames"][``state"][``slot_values"]$. Since the intent annotation ($``active intent"$) is annotated for dialog level, we ignore the intent prediction task on this dataset

The dataset provides with dialog schema, which contains possible dialog states and values for all categorical slots, we directly extract that information as the external knowledge for the DST task. The dataset also provides around 10 API results when the system side provides the requested information to the user. We sample 5 of them as the external knowledge for response generation

% We process the original SGD dataset by reformatting the dialogues and adding external knowledge. We first loop through the train, validation, and test sets, loading the data and schema files. For each dialogue, we initialize a new dialogue structure, update the dialogue history, and add annotations for both user and system turns. We then filter and accumulate candidate and offered results, while adding external knowledge for TOD, DST, and Intent. Furthermore, we transform the external knowledge into a flat string representation and generate prompts for each dialogue. Finally, we save the processed dialogues, original examples, and related files to the specified directories. This function essentially restructures the original dataset to be more suitable for the task at hand, enriching it with additional information and external knowledge.
\subsection{SimJointMovie}
\subsection{SimJointRestaurant}
\subsection{SimJointGEN}
\subsection{STAR}
\subsection{Taskmaster1}
\subsection{Taskmaster2}
\subsection{Taskmaster3}
\subsection{Wizard-of-Oz (WOZ) 2.0}
In this subsection, we processed a dialogue dataset, "WOZ2.0", for a Wizard of Oz (WOZ) task related to Dialogue State Tracking (DST). We've reformatted each dialogue with unique identifiers, user and system utterances, dialogue history, and metadata. We've also handled slot filling tasks to identify key pieces of information and incorporated external knowledge into each dialogue. Additionally, we've generated a task-specific prompt for each dialogue.

% , , , , , ,, , , , ,  ,  ,, OpenDialKG~\citep{moon2019opendialkg} and DuRecDial-2.0 \citep{liu2021durecdial}.

% Please add the following required packages to your document preamble:
% \usepackage{multirow}
\begin{table}[]
\begin{tabular}{c|l}
\hline
\multirow{17}{*}{\textbf{NLU}} & NLU++~\citep{casanueva2022nlu++} \\ 
                               & BANKING77-OOS~\citep{zhang2022pre}                                          \\ 
                               & BANKING77~\citep{casanueva2020efficient}                                              \\
                               & RESTAURANTS8K~\citep{coope2020span}                          \\
                               & CLINC150~\citep{larson2019evaluation}                                               \\
                               & CLINC-Single-Domain-OOS-banking~\citep{zhang2022pre}                        \\  
                               & CLINC-Single-Domain-OOS-credit\_cards~\citep{zhang2022pre}                 \\
                               & HWU64~\citep{liu2019benchmarking}                                                  \\
                               & SNIPS~\citep{coucke2018snips}                                                  \\
                               & SNIPS-NER~\citep{coucke2018snips}                                               \\
                               & DSTC8-SGD~\citep{coope2020span}                              \\
                               & TOP~\citep{gupta2018semantic}                                           \\
                               & TOP-NER~\citep{gupta2018semantic}                                                \\
                               & ATIS-NER~\citep{hemphill1990atis}                                               \\
                               & ATIS~\citep{hemphill1990atis}                                                   \\
                               & MIT-MOVIE~\citep{liu2013asgard}                                              \\
                               & MIT-RESTAURANT~\citep{liu2013asgard}   \\ \hline
\multirow{27}{*}{\textbf{TOD}} & KVRET~\citep{eric2017key} \\ 
                               & AirDialogue~\citep{wei2018airdialogue}                                          \\ 
                               & DSTC2-Clean~\citep{mrkvsic2017neural}                                          \\
                               & CaSiNo~\citep{chawla2021casino}                       \\
                               & FRAMES~\citep{elframes}                        \\  
                               & WOZ2.0~\citep{mrkvsic2017neural}                \\
                               & CraigslistBargains \citep{he2018decoupling}                                                \\
                               & Taskmaster1~\citep{byrne2019taskmaster}                                                 \\
                               & Taskmaster2~\citep{byrne2019taskmaster}                                               \\
                               & Taskmaster3~\citep{byrne2019taskmaster}                              \\
                               & ABCD~\citep{chen2021action}                                         \\
                               & MulDoGO~\citep{peskov2019multi}                                              \\
                               & BiTOD \citep{lin2021bitod}                                              \\
                               & SimJointGEN~\citep{shah2018building}                                                  \\
                               & SimJointMovie~\citep{shah2018building}                                               \\
                               & SimJointRestaurant~\citep{shah2018building}  \\
                               & STAR \citep{mosig2020star} \\
                               & SGD~\citep{rastogi2020towards} \\
                               & MultiWOZ2\_1~\citep{eric2020multiwoz} \\ 
                               & MultiWOZ2\_2~\citep{zang2020multiwoz} \\
                               & HDSA-Dialog~\citep{chen2021action} \\
                               & MS-DC~\citep{li2018microsoft} \\
                               & GECOR~\citep{quan2019gecor} \\
                               & Disambiguation~\citep{qian2022database} \\
                               & MetaLWOZ~\citep{lee2019multi} \\
                               & KETOD~\citep{chen2022ketod} \\
                               & MuDoCo~\citep{martin2020mudoco} \\ \hline
  \multirow{1}{*}{\textbf{Conv-Rec}} & SalesBot~\citep{chiu2022salesbot} \\                              
\end{tabular}
\end{table}
